# Supplementary material for: Local Minima Structures in Gaussian Mixture Models
Source: arXiv:2009.13040 source file (2024-03-09)
Supplement: Supplementary file 1 [file AppxZ_additional.tex]

\DG{It remains to show an upper bound for each term above, i.e., $\left\| \sum_{s \in \cB_{i,j}} \E_s[\Asso_i] \cdot \big( \bv_s - \bbeta_i \big) \right\|$ is ``small.''}

=====================

\DG{This is under construction:}

Let $s \in \cB_{ij}$ and recall that $\bv_s = \E_s \left[ \frac{\Asso_i}{\E_s[\Asso_i]} \cdot \sfx \right]$. 
We want to show $\big\| \E_s[\Asso_i] \cdot (\bv_s - \bbeta_i ) \big\|$ is small. 

\begin{figure}[t]
    \centering
    \begin{tikzpicture}
        \draw (-2,-3.5) -- (-2,1);
        \draw[dashed] (-6,-2) -- (2,-2);

        \filldraw[black] (-6,-2) circle (2pt) node[anchor=north] {$\bbeta_i$};
        \filldraw[black] (2,-2) circle (2pt) node[anchor=north] {$\bbeta_j$};

        \ngram{0.1}{7}{45}{thick,fill=red};
        \draw (0.3, 0.3) node {$\bthetastar_s$};
        %\filldraw[black] (2,2) star (2pt) 

        \draw (-6, -3.1) -- (-6, -2.9);
        \draw (2, -3.1) -- (2, -2.9);
        \draw[<->, dotted, thick] (-6,-3) -- (2,-3);
        \draw (-1.5, -3) node[anchor=north] {$d_{ij}$};

        \draw (-2, -2.4) -- (-2, -2.2);
        \draw (0, -2.4) -- (0, -2.2);
        \draw[<->, dotted, thick] (-2,-2.3) -- (0,-2.3);
        \draw (-0.8, -2.3) node[anchor=north] {$b$};

        \draw[<->, dotted, thick] (0,0) -- (0,-2);
        \draw (0, -1) node[anchor=west] {$h$};
    \end{tikzpicture}
    \caption{Illustration}
    \label{fig:illustration}
\end{figure}
Let us introduce some notation first. We may assume $i, j \in [\kfit]$, and $s \in \cB_{ij}$ are fixed from now on. 
\begin{align*}
    d_{ij} &\coloneqq \left\| \bbeta_j - \bbeta_i \right\|,\\
    b   &\coloneqq \left\| \pi_{ij} \left( \bthetastar_s - \frac{\bbeta_i + \bbeta_j}{2} \right) \right\|
        \qquad \text{where }\pi_{ij}(\bv) \coloneqq \left\langle \bv, \frac{\bbeta_j - \bbeta_i}{\|\bbeta_j - \bbeta_i} \right\rangle,\\
    h   &\coloneqq \left\| \pi_{ij}^{\perp} \left( \bthetastar_s - \frac{\bbeta_i + \bbeta_j}{2} \right) \right\|
        \qquad \text{where }\pi_{ij}^{\perp}(\bv) \coloneqq \bv - \pi_{ij}(\bv).
\end{align*}
See Figure \ref{fig:illustration} for illustration.

We assume the following for now, which we will need to formally prove as well:
\begin{enumerate}[label=\texttt{(C\arabic*)}]
    \item\label{claim:reweight}
    $\big\| \E_s[\Asso_i] \cdot (\bv_s - \bbeta_i ) \big\| \leq \big\| \E_s[\Asso_i] \cdot (\bthetastar_s - \bbeta_i ) \big\| = \E_s[\Asso_i] \cdot \big\| \bthetastar_s - \bbeta_i \big\|$

    \item\label{claim:vertical}
    $\| \pi_{ij}^{\perp} ( \bthetastar_s - \bbeta_j ) \| \leq \diam \cV_j$ where $\diam \cV_j \coloneqq \min\{ \max_{s,s' \in \vor_{j} }\|\bthetastar_s - \bthetastar_{s'}\|, ~C  \}$ ($C$ is a constant, e.g., 1).
\end{enumerate}
Then, we make two observations. 
\begin{enumerate}
    \item 
    Upper bounds on $\E_s[\Asso_i]$. We have two upper bounds:
    \begin{enumerate}
        \item 
        Recall Corollary \ref{cor:small_bdr}-claim 2 and the definition of $\setB_i^{\delta}$ in \eqref{eq:setB}, and observe that for all $s \in \setB_i^{\delta}$,
        \begin{align*}
            \E_{s}\left[\Asso_{i}\right] 
                &\leq 9 \left(\sqrt{2\pi} + 1 \right) \cdot \kfit^2 \sum_{j\in [\kfit]\setminus\{i\}} \frac{ \| \bbeta_i - \bbeta_j \| }{\sigma} \cdot \E_{s}\left[ \Asso_i \Asso_j  \right]\\
                &\leq 9 \left(\sqrt{2\pi} + 1 \right) \cdot \kfit^3 \cdot \delta.
        \end{align*}

        \item 
        Without loss of generality, we may identify $\frac{\bbeta_i + \bbeta_j}{2} = 0$ and choose a basis of $\real^d$ such that $\e_1 = \frac{\bbeta_j - \bbeta_i}{\| \bbeta_j - \bbeta_i \|}$. 
        Letting $\phi_{\std}(x) = \frac{1}{\sqrt{2\pi}} e^{-\frac{x^2}{2\std^2}}$ denote the density of $\cN(0, \std^2)$, we observe that 
        \begin{align*}
            \E_s \left[ \Asso_i \right]
                &= \int_{\real^d} \psi_i(\x) \cdot \frac{1}{ (2\pi \std^2)^{d/2}} \cdot e^{- \frac{\| \x - \bthetastar_s \|^2}{2\std^2}} ~d\x\\
                &\leq \int_{\real} \frac{ \phi_{\std}\left( x + \frac{d_{ij}}{2} \right)}{\phi_{\std}\left( x + \frac{d_{ij}}{2} \right) + \phi_{\std}\left( x - \frac{d_{ij}}{2} \right)} \cdot \phi_{\std}\left( x - b \right) ~dx\\
                &= \int_{\real} \frac{1}{1 + e^{ \frac{d_{ij} \cdot x}{\sigma^2}}} \cdot \phi_{\std}(x-b) ~dx \\
                &\leq \int_{-\infty}^{0} \phi_{\std}( x - b ) ~dx + \int_0^{\infty} e^{ -\frac{d_{ij} \cdot x}{\sigma^2}} \cdot \phi_{\std}(x-b) ~dx\\
                &= Q\left( \frac{b}{\std}\right) 
                    + e^{\frac{d_{ij}( d_{ij} - 2b)}{2\std^2}} \cdot Q \left( \frac{d_{ij} - b}{\std} \right).
                %&\leq \left( 1 + \frac{4 \std}{\sqrt{2\pi} \cdot \min\{2b, d_{ij}\} } \right) e^{- \frac{\min\{2b, d_{ij}\}^2}{32 \sigma^2}}.
                    % &&\because \text{Lemma \ref{lem:Psi_domination}}
        \end{align*}
        Since $Q(t) \leq \frac{Q(0)}{\phi(0)} \phi(t) = \sqrt{\frac{\pi}{2}}\cdot \phi(t)$ for all $t \geq 0$, 
        \begin{align*}
            &\text{if }b \leq d_{ij},
                &\E_s \left[ \Asso_i \right] &\leq \sqrt{\frac{\pi}{2}} \cdot \left[ \phi\left( \frac{b}{\std}\right) + e^{\frac{d_{ij}( d_{ij} - 2b)}{2\std^2}} \cdot \phi\left( \frac{d_{ij} - b}{\std} \right) \right]\\
                    &&&= \sqrt{2\pi} \cdot \phi\left( \frac{b}{\std}\right)\\
                    &&&=e^{-\frac{ b^2}{2\std^2}},\\
            &\text{if }b > d_{ij},
                &\E_s \left[ \Asso_i \right] &\leq \sqrt{\frac{\pi}{2}} \cdot \phi\left( \frac{b}{\std}\right) + e^{\frac{d_{ij}( d_{ij} - 2b)}{2\std^2}} 
                    &&\because Q \left( \frac{d_{ij} - b}{\std} \right) \leq 1\\
                &&&\leq \frac{1}{2} e^{- \frac{b^2}{2 \sigma^2}} + e^{- \frac{d_{ij} \cdot b}{2 \sigma^2}}
                    &&\because d_{ij} - b < 0\\
                &&&\leq 2 e^{-\frac{ d_{ij} \cdot b}{2\std^2}}.
        \end{align*}
    \end{enumerate}

    \item 
    An upper bound on $\big\| \bthetastar_s - \bbeta_i \big\|$.
    \begin{align}
        \big\| \bthetastar_s - \bbeta_i \big\|
            &= \sqrt{ \left( \frac{d_{ij}}{2} + b \right)^2 + h^2 } &&\because\text{Pythagorean theorem}
                \nonumber\\
            &\leq \sqrt{ \left( \frac{d_{ij}}{2} + b \right)^2 + (\diam \cV_j)^2 }  && \because \ref{claim:vertical}    \nonumber\\
            &\leq \frac{d_{ij}}{2} + b + \diam \cV_j.     &&\because \sqrt{A + B} \leq \sqrt{A} + \sqrt{B}
    \end{align}
\end{enumerate}

We consider the two cases, (1) $b \leq d_{ij} / 2$ and (2) $b > d_{ij}/2$ separately.

\begin{itemize}
    \item 
    \textit{Case 1. $b \leq d_{ij} / 2$.}

\end{itemize}

=====================
\clearpage
For simplicity, let me assume $\std = 1$ for now. 
Suppose that $s \in \cB_{ij} \subset \setB_i^{\delta}$. 
We want to show that
\[
    \E_s\left[ \Asso_i \right] \cdot d_{ij} \lesssim \delta
\]
where $d_{ij} \coloneqq \| \bbeta_i - \bbeta_j \|$. 
To prove this claim, I conjecture it would suffice to show that either of the following:
\begin{equation}\label{eqn:conj1}
    d^*_s \coloneqq d( \bthetastar_s, \vor_i ) \gtrsim \sqrt{ \log \left( \frac{1}{\delta} \right)}
\end{equation}
or 
\begin{equation}\label{eqn:conj2}
    \tilde{d}^*_s \coloneqq \min_{j' \in [\kfit]\setminus\{i\}} \left\langle \bthetastar_s - \frac{\bbeta_i + \bbeta_{j'}}{2}, \frac{\bbeta_{j'} - \bbeta_i}{\|\bbeta_{j'} - \bbeta_i\|} \right\rangle \gtrsim \sqrt{ \log \left( \frac{1}{\delta} \right)}.
\end{equation}
\DG{I don't know which inequality is the right one to show. 
I think \eqref{eqn:conj1} is likely true, but we may need to show a stronger inequality, e.g., in \eqref{eqn:conj2}, however, it may not be true.}
In the rest of the argument on this page, let $d^*$ denote the quantity, whether it be $d^*_s$ or $\tilde{d}^*_s$.

Without loss of generality, we may assume $\frac{\bbeta_i + \bbeta_j}{2} = 0$ and $\e_1 = \frac{\bbeta_j - \bbeta_i}{\|\bbeta_j - \bbeta_i\|}$. 
We make two observations:
\begin{enumerate}
    \item 
    By definition, cf. \eqref{eq:setB}, 
    \begin{equation}\label{eqn:cond}
        \max_{j'} \| \bbeta_i - \bbeta_{j'}\| \cdot \E_s[\Asso_i \Asso_{j'}] < \delta.
    \end{equation}
    Therefore,
    \[
        \sum_{j' \in [\kfit]\setminus\{i\}} \E_s\left[ \Asso_i \Asso_j \right] 
            < \sum_{j' \in [\kfit]\setminus\{i\}} \frac{\delta}{\|\bbeta_i - \bbeta_{j'}\|}
            \leq \frac{ (\kfit - 1 )\delta}{ \min_{j' \in[\kfit]\setminus\{i\}} \|\bbeta_i - \bbeta_{j'}\|}.
    \]

    \item 
    Observe that 
    \[
        \sum_{j' \in [\kfit]\setminus\{i\}} \asso_{j'}(\x)
            = 1 - \psi_i(\x)
            \geq \frac{1}{2} \cdot \indic\{\x \in \vor^c_i\}
    \]
    where $\vor_i = \{ \x \in \real^d: \| \x - \bbeta_i \| \leq \| \x - \bbeta_{j'}\|, ~\forall j' \in [\kfit] \}$. 
    Thus,
    \begin{align*}
        \sum_{j' \in [\kfit]\setminus\{i\}} \E_s\left[ \Asso_i \Asso_{j'} \right] 
            = \E\left[ \Asso_i \cdot ( 1 - \Asso_i ) \right]
            \geq \frac{1}{2} \E\big[ \Asso_i \cdot \indic\{\sfx \in \vor^c_i\} \big]
    \end{align*}
\end{enumerate}

Suppose that we can show that 
\begin{equation}\label{eqn:conj_to_show}
    \E\big[ \Asso_i \cdot \indic\{\sfx \in \vor^c_i\} \big] 
        \gtrsim \frac{ 1 }{ \min_{j' \in[\kfit]\setminus\{i\}} \|\bbeta_i - \bbeta_{j'}\|} \cdot e^{ - {d^*}^2}.
\end{equation}
Then it follows that 
\[
    d^* \gtrsim \sqrt{ \log \left( \frac{1}{\kfit \cdot \delta} \right)}.
\]

Now, the remaining question is how to establish \eqref{eqn:conj_to_show}, or something similar.

Two possible approaches:
\begin{enumerate}
    \item 
    \textit{Approach 1.} 
    Decompose $\x \in \real^d$ as  $\x = (x_1, \x_2)$ where $x_1 \in \real$ and $\x_2 \in \real^{d-1}$. 
    For each $l \in [\kfit]$, write $\bbeta_l = (a_l, \b_l)$ where $a_l \in \real$ and $\b_l \in \real^{d-1}$. In particular, $\bbeta_i = (-R, 0)$ and $\bbeta_j = (R, 0)$.
    Observe that 
    \begin{align*}
        \psi_i(\x) 
            &= \frac{e^{- \frac{1}{2}\|\x - \bbeta_i \|^2}}{\sum_{l \in [\kfit]} e^{- \frac{1}{2}\|\x - \bbeta_l \|^2 }}\\
            &= \frac{1}{\sum_{l \in [\kfit]} e^{ \left\langle \bbeta_l - \bbeta_i, \x - \frac{\bbeta_i + \bbeta_l}{2} \right\rangle } }\\
            &=\frac{1}{\sum_{l \in [\kfit]} e^{(a_l + R) x_1} \cdot e^{\langle \b_l, \x_2 \rangle} \cdot e^{-\frac{1}{2} \big( \| \bbeta_l \|^2 - R^2 \big)} }\\
            &\geq e^{-(a_{\max} + R) x_1} \cdot \frac{1}{\sum_{l \in [\kfit]} e^{\langle \b_l, \x_2 \rangle} \cdot e^{-\frac{1}{2} \big( \| \bbeta_l \|^2 - R^2 \big)} }
                \qquad \text{where}\quad a_{\max} \coloneqq \max_{l \in [\kfit]} a_l.
    \end{align*}

    Next, we draw on our argument for the simple case with $d=1$ and $k=2$ to obtain
    \begin{align*}
        \E\big[ \Asso_i \cdot \indic\{\sfx \in \vor^c_i\} \big] 
            &= \int_{x_1 \in \real} \int_{\x_2 \in \real^{d-1}} \psi_i(\x) \cdot \indic\{\sfx \in \vor^c_i\} \cdot \frac{1}{\sqrt{2\pi}} e^{-\frac{(x_1 - \theta^*_1)^2}{2}} \cdot \frac{1}{(2\pi)^{\frac{d-1}{2}}} e^{-\frac{\|\x_2 - \theta^*_2\|^2}{2}} ~ dx_1 d\x_2\\
            &\geq \left( \int_0^{\infty} e^{-(a_{\max} + R) x_1} \cdot \frac{1}{\sqrt{2\pi}} e^{-\frac{(x_1 - \theta^*_1)^2}{2}}  ~dx_1 \right)\\
                &\qquad \times  \underbrace{\left( \int_{\real^{d-1}}  \frac{1}{\sum_{l \in [\kfit]} e^{\langle \b_l, \x_2 \rangle} \cdot e^{-\frac{1}{2} \big( \| \bbeta_l \|^2 - R^2 \big)} } \cdot  \frac{1}{(2\pi)^{\frac{d-1}{2}}} e^{-\frac{\|\x_2 - \theta^*_2\|^2}{2}} ~d\x_2 \right)}_{\eqqcolon (*)}
    \end{align*}
    \DG{Challenge: Establishing a lower bound for (*) seems not easy. In particular, it can get very small when $\theta^*_2$ is close to some $\bbeta_l$ with $\l \in [\kfit] \setminus \{i, j\}$.  While this is actually a favorable setting for our eventual goal to show $\E_s[\Asso_i] \cdot d_{ij} \lesssim \delta$, I don't know how to formally complete the argument. }

    \item 
    \textit{Approach 2.} 
\end{enumerate}

=========
\clearpage
\DG{Nov 2, 2023}
\paragraph{Second Attempt for Proof of Proposition \ref{prop:small_bdr2}.}

We are trying to upper bound $\big\| \hbbeta_i - \bbeta_i \big\|$ where
\[
    \hbbeta_i
        \coloneqq \sum_{s \in [\ktrue]} \hw_s \cdot \hbv_s
        =\frac{1}{|\setA_i^{\delta}|} \sum_{s \in \setA_i^{\delta}} \bthetastar_s,
        \qquad\text{and}\qquad
    \bbeta_i
        = \frac{\E_*[ \Asso_i \sfx]}{\E_*[ \Asso_i ]}
        = \sum_{s \in [\ktrue]} \underbrace{\frac{ \E_s[\Asso_i]}{ \sum_{s \in [\ktrue]} \E_s[\Asso_i]}}_{\eqqcolon w_s} \cdot \underbrace{\E_s \left[ \frac{\Asso_i}{\E_s[\Asso_i]} \cdot \sfx \right]}_{\eqqcolon\bv_s}.
\]

After a few lines of algebra, based on \eqref{eqn:beta_p}, \eqref{eqn:beta_pp} and \eqref{eqn:prop4_step1}, we would obtain
\begin{align*}
    \big\| \hbbeta_i - \bbeta_i \big\|
        &\leq \frac{\kfit \cdot \bdw}{1 - \kfit \cdot \bdw} \cdot \left( \min_{s \in \setA_i^{\delta}} \max_{s' \in \setA_i^{\delta}} \| \bthetastar_s - \bthetastar_{s'} \| + 3 \cdot \std \right)
            &&\because \eqref{eqn:prop4_step2A}\\
            &\quad+ \frac{1}{\sum_{s \in \setA_i^{\delta}} \E_s[\Asso_i]} \cdot \sum_{j \in [\kfit]\setminus\{i\}} \left\| \sum_{s \in \cB_{i,j}} \E_s[\Asso_i] \cdot \big( \bv_s - \bbeta_i \big) \right\|
            +  \frac{1}{\sum_{s \in \setA_i^{\delta}} w_s} \cdot \sum_{s \in \setC_i^{\delta}} w_s \cdot \big\| \bv_s - \bbeta_i \big\|
\end{align*}
where $\setC_i^{\delta} \coloneqq [\ktrue] \setminus \big( \setA_i^{\delta} \cup \setB_i^{\delta} \big)$. Recall that by Lemma \ref{lem:A_or_B}, $|\setC_i^{\delta}| = 0$ or $|\setC_i^{\delta}| = 1$. 

At the end of the day, the question reduces to establishing an upper bound for 
\begin{equation}
     \left\| \sum_{s \in \cB_{i,j}} \E_s[\Asso_i] \cdot \big( \bv_s - \bbeta_i \big) \right\|
\end{equation}
for each $j \neq i$, where we recall from \eqref{eqn:residual_term} that
\begin{equation}
    \setB_{i,j} 
        = \left\{ s \in [\ktrue] ~\bigg|~ \iota_{\B}(\bthetastar_s) = j ~~~\text{and}~~ \max_{j' \in [\kfit]}  \frac{ \| \bbeta_i - \bbeta_{j'} \| }{\sigma} \cdot  \E_s \left[ \Asso_i \Asso_{j'} \right] < \delta \right\}.
\end{equation}

\subparagraph{Two useful lemmas.}
To proceed, we state and prove two lemmas.
\begin{lemma}\label{lem:single_asso}
    For any $(i,s) \in [\kfit] \times [\ktrue]$ and any $\alpha \geq 0$,
    \[
        \E_s \big[ \Asso_i \big] 
                \leq  \P_s\left( \softvor^{\alpha}_i \right) + e^{-\alpha \cdot \frac{ d^{\min}_i}{\std}}. \label{eq:conj2_1}
    \]
    where $d^{\min}_i \coloneqq  \min_{j \in [\kfit]\setminus\{i\}} \|\bbeta_{j}-\bbeta_i\|$.
\end{lemma}
\begin{proof}[Proof of Lemma \ref{lem:single_asso}]
    Recall from \eqref{eqn:alpha_enlarged} that 
    \[
        \softvor_{i}^{\alpha} 
            \coloneqq\left\{ \x \in \real^d :\left\langle \x-\bbetabar_{ij},~\frac{\bbeta_{i}-\bbetabar_{ij}}{\|\bbeta_{i}-\bbetabar_{ij}\|}\right\rangle \ge-\alpha \sigma,~~\forall j\in[\kfit]\setminus\{i\}\right\}
            \qquad\text{where}\quad \bbetabar_{ij} = \frac{\bbeta_i + \bbeta_j}{2}.
    \]
    Thus, 
    \[
        \x \not\in \softvor_{i}^{\alpha}
            \qquad\implies\qquad
            \exists j \in[\kfit]\setminus\{i\} ~~\text{such that}~~
            \left\langle \frac{\x-\bbetabar_{ij}}{\std},~\frac{\bbeta_{j}-\bbeta_i}{\std} \right\rangle \ge \alpha \cdot \frac{\|\bbeta_{j}-\bbeta_i\|}{\std}.
    \]
    For any $\alpha \geq 0$, we observe that if $\x \not\in \softvor^{\alpha}_i$, then
    \begin{align*}
        \asso_i(\x) 
            \leq \min_{j \in [\kfit]\setminus\{i\}} \frac{\phi_i(\x)}{\phi_i(\x) + \phi_j(\x)}
            = \min_{j \in [\kfit]\setminus\{i\}} \frac{1}{1 + e^{\big\langle \frac{\x-\bbetabar_{ij}}{\std},~\frac{\bbeta_{j}-\bbeta_i}{\std} \big\rangle}}
            \leq \frac{1}{1 + e^{\alpha \cdot \frac{ d^{\min}_i}{\std}}}
            \leq e^{-\alpha \cdot \frac{ d^{\min}_i}{\std}}.
    \end{align*}
    Thus, it follows that
    \begin{align*}
        \E_s \big[ \Asso_i \big] 
            &= \E_s \big[ \Asso_i \cdot \indic\{ \sfx \in \softvor^{\alpha}_i\} \big] + \E_s \big[ \Asso_i \cdot \indic\{ \sfx \not\in \softvor^{\alpha}_i\} \big]
            \leq \P_s\left( \softvor^{\alpha}_i \right) + e^{-\alpha \cdot \frac{ d^{\min}_i}{\std}}.
    \end{align*}
\end{proof}

\begin{lemma}\label{lem:double_asso}
    For any $(i,j,s) \in [\kfit] \times [\kfit] \times [\ktrue]$ such that $i \neq j$ and any $\alpha \geq 0$,
    \[
        \P_s\left( \softvor_{i}^{\alpha} \cap \softbdr_{ij}^{\alpha} \right) 
            \leq \kfit^2 \cdot \exp \left( 3\alpha \frac{ \| \bbeta_i - \bbeta_j \| }{\sigma} \right) \cdot \E_s \big[ \Asso_i \Asso_j \big]. \label{eq:conj2_2}
    \]
    where $d^{\min}_i \coloneqq  \min_{j \in [\kfit]\setminus\{i\}} \|\bbeta_{j}-\bbeta_i\|$.
\end{lemma}
\begin{proof}[Proof of Lemma \ref{lem:double_asso}]
    Recall from \eqref{eq:goodset} that for any $\delta > 0$ and $i, j \in [\kfit]$ with $i \neq j$,  
    \[
        \goodset_{ij}^{\delta}:=\left\{ \x \in \real^d :\asso_{i}(\x)\asso_{j}(\x)\ge \delta \right\}.
    \]
    Thus, we have
    \begin{equation}\label{eqn:double.1}
        \E_s \big[ \Asso_i \Asso_j \big]
            = \E_s \big[ \Asso_i \Asso_j \cdot \indic\{ \sfx \in \goodset_{ij}^{\delta} \} \big] + \E_s \big[ \Asso_i \Asso_j \cdot \indic\{ \sfx \not\in \goodset_{ij}^{\delta} \} \big]
            \geq \delta \cdot \P_s\big( \goodset_{ij}^{\delta} \big)
    \end{equation}
    By Claim 3 of Lemma \ref{lem:geometry}, cf. the inclusion \eqref{eq:geometry3}, we observe that for any $\alpha \in \real$,
    \[
        \P_s\big( \softvor_{i}^{\alpha} \cap \softbdr_{ij}^{\alpha} \big) 
            \leq \P_s\big( \goodset_{ij}^{\delta'} \big) 
            \leq \frac{1}{\delta'} \E_s \big[ \Asso_i \Asso_j \big]
            \qquad\text{where}\quad
            \delta' = \frac{1}{\kfit^2} \exp \left( - 3\alpha \frac{ \| \bbeta_i - \bbeta_j \| }{\sigma} \right).
    \]
\end{proof}

\subparagraph{To assemble these lemmas.} 
Informally, we are aiming to show that
\[
    \E_s\big[ \Asso_i \big] \lesssim \frac{\delta}{\| \v_s - \bbeta_i\|}.
\]
Using Lemmas \ref{lem:vol_intersect}, \ref{lem:single_asso}, and \ref{lem:double_asso}, we obtain that for any $\alpha > 0$ and $\alpha'_j > 0, ~\forall j \in [\kfit]\setminus\{i\}$,
\begin{align*}
    \E_s \big[ \Asso_i \big] 
        &\leq  \P_s\left( \softvor^{\alpha}_i \right) + e^{-\alpha \cdot \frac{ d^{\min}_i}{\std}}
            &&\because\text{Lemma \ref{lem:single_asso}}\\
        &\leq \left(\sqrt{2\pi} + 1 \right) \sum_{j\in [\kfit]\setminus\{i\}} \max\left\{ 1, ~\frac{1}{\alpha'_j} \right\} \cdot  \P_{s}\left(\softvor_{i}^{\alpha + \alpha'_j}\cap\softbdr_{ij}^{\alpha + \alpha'_j}\right)
            &&\because\text{Lemma \ref{lem:vol_intersect}}\\
            &\qquad\qquad\qquad\text{\DG{revision/verification required}}\\
        &\leq \left(\sqrt{2\pi} + 1 \right) \kfit^2 \sum_{j\in [\kfit]\setminus\{i\}} \max\left\{ 1, ~\frac{1}{\alpha'_j} \right\} \cdot  \exp \left( 3 (\alpha + \alpha'_j) \frac{ \| \bbeta_i - \bbeta_j \| }{\sigma} \right) \cdot \E_s \big[ \Asso_i \Asso_j \big]
            &&\because\text{Lemma \ref{lem:double_asso}}
\end{align*}
By definition of $\setB_{i,j}$, we have $\max_{j' \in [\kfit]\setminus\{i\}}  \frac{ \| \bbeta_i - \bbeta_{j'} \| }{\sigma} \cdot  \E_s \left[ \Asso_i \Asso_{j'} \right] < \delta$, and therefore, with the choice of $\alpha, \alpha'_j \asymp \frac{\std}{\|\bbeta_i - \bbeta_j\|}$, we get $\E_s\big[\Asso_i\big] \lesssim \kfit^3 \cdot \delta$.
\DG{I think this is not sufficient as $\|v_s - \bbeta_i\|$ can be large. The question is whether we can improve Lemma \ref{lem:vol_intersect} using the updated version of Lemma \ref{lem:gaussian_property}, along with the additional (trivial) upper bound in Lemma \ref{lem:gaussian_upper} to handle the case where $\alpha'_j$ is small...}

\clearpage
\DG{Updated on November 3}
\begin{enumerate}
    \item 
    ((Im-)Possibility of improving Lemma \ref{lem:gaussian_property}) 
    Recall what we want to show: given $t_1, t_2, \tau$ such that $0 \leq t_1 \leq t_2 \leq \infty$ and $\tau > 0$, we want
    \[
        \int_{t_1}^{t_2} \phi(z) dz \leq C(t_1, \tau) \cdot \int_{t_1}^{t_1+\tau} \phi(z) dz.
    \]
    with $C(t_1, \tau) \asymp \frac{1}{t_1 \tau}$. The candidate argument we discussed goes as follows:
    \begin{align}
        \int_{t_1}^{t_2} \phi(z) dz
            &\leq \int_{t_1}^{\infty} \phi(z) dz
                = Q(t_1)\\
            &\leq \frac{1}{t} \phi(t_1)
                \leq \frac{e^{\tau (t_1 + \frac{1}{2}\tau)}}{t_1} \phi(t_1 + \tau)\\
            &\leq \underbrace{\frac{e^{\tau (t_1 + \frac{1}{2}\tau)}}{t_1 \tau}}_{\geq e \cdot e^{\frac{1}{2}\tau^2}} \int_{t_1}^{t_1+\tau} \phi(z) dz \label{eq:conj0}
    \end{align}
    Thus, this provides us an even worse upper bound than that in Lemma \ref{lem:gaussian_property}.
    \YC{Not always worse. When $\tau=1/d_{ij}$ and $d_{ij}$ is large (the regime of concern), $e^{\tau^2}=O(1)$ is better than $\frac{1}{\tau}$ in Lemma \ref{lem:gaussian_property}.}
    \DG{If we revisit the proof of Lemma \ref{lem:gaussian_property}, we can see  it is possible to prove something like
    $C(t_1, \tau) \asymp (1 + \frac{1}{t_1}) \cdot \max\Big\{1, \frac{1}{\tau}\Big\}$, but I don't think we can remove that $1$ added to $\frac{1}{t_1}$.} \YC{Here we have an additional factor $e^{\tau (t_1+\tau)} \approx e^{\tau t_1}$ in \eqref{eq:conj0}. If $t_1 \le 10 d_{ij} \asymp \frac{1}{\tau}  $, then this factor is just a constant. If $t_1 \ge  10 d_{ij}$, then I think we would have $\|\theta_s^* - \beta_i\| \lesssim \Delta_{new} := \|\theta_s^* -\beta_j\|$, a favorable case for us. In fact, when $t_1\ge d_{ij}$ is so large, it may be more direct to use the bound 
    \begin{equation}
         \int_{t_1}^{t_2} \phi(z) dz
            \leq \int_{t_1}^{\infty} \phi(z) dz
            \lesssim e^{-t_1^2} \ll \frac{1}{d_{ij}}.
    \end{equation}}
    
    \item 
    For each $j \neq i$ and each $s \in \setB_{i,j} $,
    \begin{align}
        \E_s[\Asso_i] \cdot \big( \bv_s - \bbeta_i \big)
            = \E_s \big[ \Asso_i \cdot ( \sfx - \bbeta_i ) \big]
    \end{align}
    \DG{
    We want to relate $\E_s \big[ \Asso_i \cdot ( \sfx - \bbeta_i ) \big]$ to $\max_{j' \in [\kfit]}  \| \bbeta_i - \bbeta_{j'} \| \cdot  \E_s \left[ \Asso_i \Asso_{j'} \right]$...
    }
    \begin{itemize}
        \item 
        \textbf{Conjecture 1:} $ \big\| \E_s \big[ \Asso_i \cdot ( \sfx - \bbeta_i ) \big] \big\| \leq  \E_s \big[ \Asso_i \big] \cdot \big\| \bthetastar_s - \bbeta_i \big\|$
        \item 
        \textbf{Conjecture 2:} 
        We want to show 
        \begin{equation}
        \E_s \big[ \Asso_i \big] \leq C \cdot \max_{j' \neq i} \E_s \big[ \Asso_i \cdot \Asso_{j'} \big].
        \label{eq:conj2_0}
        \end{equation}
        \YC{I do not expect this to hold for a constant $C$ (I am treating $\kfit$ as a constant). Instead, $C$ may depend on $1/t_1$ for the $t_1$ in Lemma \ref{lem:gaussian_property}. Here $t_1$ corresponds to the distance between $\theta_s^*$ and $\partial_{ij}$ in the direction of $\beta_i - \beta_j$. I am hoping that 
        \begin{itemize}
            \item either $t_1$ is large and so that $1/t_1$ can cancel out $1/\tau \approx 1/\alpha_i \approx d_{ij}$ in Lemmas \ref{lem:gaussian_property} and~\ref{lem:vol_intersect}, or
            \item $t_1$ is small so $\|\theta_s^* - \beta_i\|$ is comparable to $\Delta_{new} = \|\theta_s^* -\beta_j\|.$
        \end{itemize} }
        To this end, it suffices to show
        \begin{align}
            \E_s \big[ \Asso_i \big] 
                &\leq C_1 \cdot \P_{s}\left(\vor_{i}\right) \label{eq:conj2_1}\\
            \P_{s}\left(\softvor_{i}^{\alpha_j}\cap\softbdr_{ij}^{\alpha_j'}\right)
                &\leq C_2 \cdot \E_s \big[ \Asso_i \cdot \Asso_{j'} \big]   \qquad\text{for appropriate }\alpha> 0. \label{eq:conj2_2}
        \end{align} 
        \DG{It is unclear to me how to prove these...}
        \YC{For~\eqref{eq:conj2_2}, can we use Lemma~\ref{lem:geometry} Part 3, which says that the value of $\psi_i\psi_j$ is large on the set $\softvor_{i}^{\alpha_j}\cap\softbdr_{ij}^{\alpha_j'}$?
        For~\eqref{eq:conj2_1}, perhaps we should expect something like 
        \[\E_s \big[ \Asso_i \big]  = \E_s \big[ \Asso_i \indic\{\sfx \in \softvor_{i}^{\alpha}\} \big] + \E_s \big[ \Asso_i \indic\{\sfx \not\in \softvor_{i}^{\alpha}\} \big] 
                \leq C_1 \cdot \P_{s}\left(\softvor_{i}^{\alpha}\right) + \epsilon 
        \] by using   Lemma~\ref{lem:geometry} Part 1 and a large enough $\alpha$ so that $\epsilon$ is negligible (say $\epsilon \le 1/d_{ij}$?).
        }\\
        \YC{Added Nov 8: The approach in the last display equation may not work, since for $\epsilon$ to be small, we need to choose $\alpha$ to be large enough that $\psi(x)\lesssim 1/d_{ij}$ is small for $x \not\in \softvor_{i}^{\alpha} $. However, this also means that $\psi(x)$ is small near the boundary of $\softvor_{i}^{\alpha}$, which may mess up the proof of \eqref{eq:conj2_2} for which we need $\psi_i\psi_j$ to be $\gtrsim 1$.}
        \YC{Following up on the above: Instead, we can try to use a more efficient bound:
        \begin{align}
            \E[\Psi_{i}] & =\E\left[\Psi_{i}\indic\{x\in\vor_{j}\}\right]+\E\left[\Psi_{i}\indic\{x\in\vor_{i}\}\right]\\
            & \le\E\left[(k\Psi_{j})\Psi_{i}\indic\{x\in\vor_{j}\}\right]+\P\{x\in\vor_{i}\} &  & \psi_{j}(x)\ge\frac{1}{\kfit}\text{ for }x\in\vor_{j}\\
            & \le\kfit\E\left[\Psi_{j}\Psi_{i}\right]+\P\{x\in\vor_{i}\}.
        \end{align}
        Note that for the 1st RHS term, we avoided using $\softvor_{i}^{\alpha}$ to bridge $\Psi_i$ and $\Psi_i\Psi_j$, so that we do not need to deal with $\alpha.$ Also note that this argument rely on $\kfit = 2$.
        }
    \end{itemize}

    \item
    Since we know $s \in \setB_{i,j} \implies \iota_{\B}(\bthetastar_s) = j$, we might be able to show that for a sufficiently small $a \geq 1$ and $C \geq 1$,
    \begin{equation}
        \E_s[ \Asso_i \Asso_j ] \geq \frac{C}{k^a}\cdot \E_s[ \Asso_i ].
    \end{equation}
    \DG{Rationale: with $\alpha = \sqrt{a \log k}$,
    \begin{equation}
        \E_s[ \Asso_i \Asso_j ]
            = \E_s\big[ \Asso_i \Asso_j \cdot \indic\{\sfx \in \softvor_{j}^{\alpha}\}\big] + \underbrace{\E_s\big[ \Asso_i \Asso_j \cdot \indic\{\sfx \not\in \softvor_{j}^{\alpha}\}\big]}_{\text{``small''}}
            \geq \frac{1}{k^a} \E_s\big[ \Asso_i \cdot \indic\{\sfx \in \softvor_{j}^{\alpha}\}\big].
    \end{equation}
    } 
    \YC{The high-level spirit in this Option 2 seems similar to Option 1 above, namely, using the fact that $\psi_i$ is large (resp.\ small) inside (resp.\ outside) $\softvor_{i}$, and a similar statement for $\psi_j$.} 
\end{enumerate}

=========
\clearpage
\clearpage
By triangle inequality,
\begin{equation}
    \left\| \hbbeta_i - \bbeta_i \right\|
        \leq \left\| \hbbeta_i - \tbbeta_i \right\| + \left\| \tbbeta_i - \bbeta_i \right\|.
\end{equation}
It suffices to prove upper bounds for the two terms separately. 
In the remainder of this step, we may assume $\bbeta_i = \bzero$ without loss of generality.

Firstly, we observe that
\begin{equation}\label{eqn:tilde_w}
    \tbbeta_i =  \sum_{s \in \setA_i^{\delta} \cup \setB_i^{\delta}} \tw_s \cdot \bv_s
    \qquad\text{where}\qquad
    \tw_s = \frac{ \E_s[\Asso_i]}{ \sum_{s \in \setA_i^{\delta} \cup \setB_i^{\delta}} \E_s[\Asso_i]}.
\end{equation}
Then decompose $\hbbeta_i - \tbbeta_i$ as follows:
\begin{align}
    \hbbeta_i - \tbbeta_i
        &= \sum_{s \in \setA_i^{\delta}} \big( \hw_s \cdot \hbv_s - \tw_s \cdot \bv_s \big) - \sum_{s \in \setB_i^{\delta}} \tw_s \cdot \bv_s
            \nonumber\\
        &= \sum_{s \in \setA_i^{\delta}} \big( \hw_s - \tw_s \big) \cdot  \hbv_s 
            + \sum_{s \in \setA_i^{\delta}} \tw_s \cdot \big( \hbv_s - \bv_s \big)
            - \sum_{s \in \setB_i^{\delta}} \tw_s \cdot \bv_s.
                \label{eqn:hat_tilde}
\end{align}

We let $\bdw \coloneqq 9 \left(\sqrt{2\pi} + 1 \right) \cdot \kfit^3 \cdot \delta$, to avoid cluttered notation. 
Recall from Corollary \ref{cor:small_bdr} and Proposition \ref{prop:exclusive} that if $\delta \leq \frac{1}{4 \kfit \cdot \bdw} = \frac{1}{36 \left(\sqrt{2\pi} + 1 \right) \cdot \kfit^4}$, then
\begin{align}
    1 - \E_s[ \Asso_i ] &\leq 9 \left(\sqrt{2\pi} + 1 \right) \cdot \kfit^4 \cdot \delta = \kfit \cdot\bdw,
        &&\forall s \in \setA_i^{\delta},
            \label{eqn:bdw_A}\\
    \E_s[ \Asso_i ] &\leq 9 \left(\sqrt{2\pi} + 1 \right) \cdot \kfit^3 \cdot \delta = \bdw,
        &&\forall s \in \setB_i^{\delta}.
            \label{eqn:bdw_B}
\end{align}
The norm of the three terms in \eqref{eqn:hat_tilde} can be separately bounded as follows.
\begin{itemize}
    \item 
    \textit{First term in \eqref{eqn:hat_tilde}.} 
    By \eqref{eqn:tilde_w} and \eqref{eqn:bdw_A}, for each $s \in \setA_i^{\delta}$,
    \[
        \frac{1 - \kfit \cdot \bdw}{|\setA_i^{\delta}| + |\setB_i^{\delta}|\cdot\bdw} \leq \tw_s \leq \frac{1}{|\setA_i^{\delta}| \cdot (1- \kfit \cdot \bdw)}.
    \]
    Therefore,
    \[
        |\hw_s - \tw_s| \leq \frac{\bdw}{|\setA_i^{\delta}|} \cdot \max \left\{ \frac{\kfit}{1- \kfit \cdot \bdw}, ~ \frac{ \kfit \cdot |\setA_i^{\delta}| + |\setB_i^{\delta}|}{|\setA_i^{\delta}| + |\setB_i^{\delta}|\bdw} \right\}.
    \]
    Observing that $\hbv_s = \bthetastar_s$, we obtain
    \begin{align}
        \left\| \sum_{s \in \setA_i^{\delta}} \big( \hw_s - \tw_s \big) \cdot  \hbv_s  \right\|
            &\leq \min_{s \in \setA_i^{\delta}}\max_{s' \in \setA_i^{\delta}} \| \bthetastar_s - \bthetastar_{s'} \| \cdot \sum_{s \in \setA_i^{\delta}} \left| \hw_s - \tw_s \right|
                &&\because \text{Lemma \ref{lem:convex_discr}}
                    \nonumber\\
            &\leq \bdw \cdot \max \left\{ \frac{\kfit}{1- \kfit \cdot \bdw}, ~ \frac{ \kfit \cdot |\setA_i^{\delta}| + |\setB_i^{\delta}|}{|\setA_i^{\delta}| + |\setB_i^{\delta}|\bdw} \right\} \cdot \min_{s \in \setA_i^{\delta}}\max_{s' \in \setA_i^{\delta}} \| \bthetastar_s - \bthetastar_{s'} \|.
                \label{eqn:prop4_term1.a}
    \end{align}

    \item
    \textit{Second term in \eqref{eqn:hat_tilde}.} 
    Let $z_{\delta} \coloneqq Q^{-1}\big( 1 - \kfit \cdot \bdw \big)$. 
    Observe that
    \begin{align*}
        \left\| \sum_{s \in \setA_i^{\delta}} \tw_s \cdot \big( \hbv_s - \bv_s \big) \right\|
            &\leq \frac{1}{{ \sum_{s \in \setA_i^{\delta} \cup \setB_i^{\delta}} \E_s[\Asso_i]}}
                 \sum_{s \in \setA_i^{\delta}} \left\| \E_s \left[ \Asso_i \cdot \big( \sfx - \bthetastar_s \big) \right] \right\|
                    &&\because\text{triangle inequality}
                    \\
            &\leq \frac{|\setA_i^{\delta}| \cdot \phi( z_{\delta}) \cdot \std}{{ \sum_{s \in \setA_i^{\delta} \cup \setB_i^{\delta}} \E_s[\Asso_i]}}
                    &&\because\text{Lemma \ref{lem:deviation_bd}}
                    \\
            &\leq \frac{\phi( z_{\delta}) \cdot \std}{1 - \kfit \cdot\bdw}
                    &&\because \eqref{eqn:bdw_A}
    \end{align*}
    Furthermore, observe that if $\bdw \leq \frac{1}{4}$, then $z_{\delta} \leq -0.5$ and
    \[
        \phi( z_{\delta} ) = \phi( -z_{\delta} ) \leq \frac{z_{\delta}^2 + 1}{-z_{\delta}} Q(-z_{\bdw}) \leq 3 \bdw.
    \]
    Therefore,
    \begin{equation}\label{eqn:prop4_term1.b}
        \left\| \sum_{s \in \setA_i^{\delta}} \tw_s \cdot \big( \hbv_s - \bv_s \big) \right\|
            \leq \frac{3 \bdw \cdot \std}{1 - \kfit \cdot \bdw}.
    \end{equation}

    \item
    \textit{Third term in \eqref{eqn:hat_tilde}.} 
    Again by \eqref{eqn:bdw_A} and \eqref{eqn:bdw_B}, for each $s \in \setB_i^{\delta}$,
    \[
        \tw_s = \frac{ \E_s[ \Asso_i ]}{ \sum_{s \in \setA_i^{\delta} } \E_s[\Asso_i] + \sum_{s \in \setB_i^{\delta}} \E_s[\Asso_i] } \leq\frac{\bdw}{|\setA_i^{\delta}| \cdot (1 - \kfit \cdot\bdw)}.
    \]
    Moreover, for each $s \in \setB_i^{\delta}$, 
    \[
        \| \bv_s \| = \| \bv_s - \bbeta_i \| 
            = \left\| \E_s \left[ \frac{\Asso_i}{\E_s[\Asso_i]} \cdot \sfx \right] - \bbeta_i \right\|\\
            \leq \| \bthetastar_s - \bbeta_i \|
            \leq \deltamax. 
    \]
    Therefore,
    \begin{align}
        \left\| \sum_{s \in \setB_i^{\delta}} \tw_s \cdot \bv_s \right\|
            &\leq \frac{|\setB_i^{\delta}|}{|\setA_i^{\delta}|} \cdot \frac{\bdw}{1- \kfit \cdot \bdw} \max_{s \in \setB_i^{\delta}} \| \bv_s \|
                \nonumber\\
            &\leq \frac{|\setB_i^{\delta}|}{|\setA_i^{\delta}|} \cdot \frac{\bdw \cdot \deltamax}{1- \kfit \cdot \bdw} .
                \label{eqn:prop4_term1.c}
    \end{align}
\end{itemize}

Combining the three inequalities in \eqref{eqn:prop4_term1.a}, \eqref{eqn:prop4_term1.b}, and \eqref{eqn:prop4_term1.c} with \eqref{eqn:hat_tilde}, we obtain
\begin{align}
    \left\|  \hbbeta_i - \tbbeta_i \right\|
        &\leq \bdw \cdot \max \left\{ \frac{\kfit}{1- \kfit \cdot\bdw}, ~ \frac{\kfit \cdot |\setA_i^{\delta}| + |\setB_i^{\delta}|}{|\setA_i^{\delta}| + |\setB_i^{\delta}|\bdw} \right\} \cdot \min_{s \in \setA_i^{\delta}}\max_{s' \in \setA_i^{\delta}} \| \bthetastar_s - \bthetastar_{s'} \|
            + \frac{ 3 \bdw \cdot \std}{1 - \kfit \cdot \bdw}
            + \frac{|\setB_i^{\delta}|}{|\setA_i^{\delta}|} \cdot \frac{\bdw \cdot \deltamax}{1-\kfit \cdot \bdw}
                \nonumber\\
        &\leq \bdw \left[ \max \left\{ \frac{4}{3} \kfit, ~ \frac{\kfit \cdot |\setA_i^{\delta}| + |\setB_i^{\delta}|}{|\setA_i^{\delta}| + 1} \right\} \cdot \min_{s \in \setA_i^{\delta}}\max_{s' \in \setA_i^{\delta}} \| \bthetastar_s - \bthetastar_{s'} \| 
            + 4 \cdot \std + \frac{4}{3} \frac{|\setB_i^{\delta}|}{|\setA_i^{\delta}|} \cdot \deltamax \right].
                \label{eqn:tilde_to_hat}
\end{align}
Here, the last inequality follows from $\kfit \cdot \varepsilon \leq \frac{1}{4}$, which implies $\frac{1}{1 - \kfit \cdot \bdw} \leq \frac{4}{3}$ and $|\setB_i^{\delta}|w \bdw \leq \frac{1}{4}$.

Secondly, we consider again the two possible scenarios $|\cC_i^{\delta}| = 0$ and $|\cC_i^{\delta}| = 0$ to derive an upper bound for $\tbbeta_i - \bbeta_i$. 
If $|\cC_i^{\delta}| = 0$, $\tbbeta_i = \bbeta_i$, and thus, $\left\|\tbbeta_i = \bbeta_i\right\|=0$. 
If $|\cC_i^{\delta}| = 1$, then we let
\[
    z_{s_0} \coloneqq Q^{-1} \left( \E_{s_0}\big[ \Asso_i \big] \right)
\]
where $Q$ is the Gaussian Q-funciton, and observe that
\begin{align*}
    \left\| \tbbeta_i - \bbeta_i \right\|
        &= \frac{ \E_{s_0}[\Asso_i] }{ \sum_{s \in \setA_i^{\delta} \cup \setB_i^{\delta}} \E_{s}[\Asso_i]} \cdot \left\| \bv_{s_0} - \bbeta_i \right\|
            &&\because \eqref{eqn:tilde_true}\\
        &\leq \frac{ \E_{s_0}[\Asso_i] }{ \sum_{s \in \setA_i^{\delta} \cup \setB_i^{\delta}} \E_{s}[\Asso_i]} \cdot \left( \left\| \bv_{s_0} - \bthetastar_{s_0} \right\| + \left\| \bthetastar_{s_0} - \bbeta_i \right\| \right)  \\
        &\leq  \frac{ 1 }{ \sum_{s \in \setA_i^{\delta} \cup \setB_i^{\delta}} \E_{s}[\Asso_i]} \cdot \phi\left( z_{s_0} \right)\cdot \std
            + \frac{ \E_{s_0}[\Asso_i] }{ \sum_{s \in \setA_i^{\delta} \cup \setB_i^{\delta}} \E_{s}[\Asso_i]} \cdot \frac{2\ktrue}{\delta} \cdot \std,
                &&\because \text{Lemma }\ref{lem:deviation_bd} \text{ and Corollary }\ref{cor:proximity}
\end{align*}
since (i) $\E_{s_0}[\Asso_i] \cdot \left\| \bv_{s_0} - \bthetastar_{s_0} \right\| = \left\| \E_{s_0}[ \Asso_i \cdot (\sfx - \bthetastar_{s_0}) ] \right\|$, and (ii) $s_0 \in \cC_i^{\delta} \implies i \in \cE_s^{\delta}$. 
By Lemma \ref{eqn:bdw_A}, we obtain
\begin{align}
    \left\| \tbbeta_i - \bbeta_i \right\|
        &\leq \frac{ \std }{ |\setA_i^{\delta} | \cdot ( 1 - \kfit \cdot \bdw ) } \left( \phi( z_{s_0})  + \frac{2\ktrue}{\delta} \right)
            \nonumber\\
        &\leq \frac{4}{3}\frac{ \std }{ |\setA_i^{\delta} | } \left( \frac{1}{\sqrt{2\pi}} + \frac{2\ktrue}{\delta} \right)
            \label{eqn:tilde_to_true}
\end{align}
because $\frac{1}{1 - \kfit \cdot \bdw} \leq \frac{4}{3}$ and $\phi(z_{s_0}) \leq \frac{1}{\sqrt{2\pi}}$.

% \DG{This implies
% $\frac{\| \tbbeta_i - \bbeta_i \|}{\std} \lesssim \frac{1}{|\setA_i^{\delta}|} \left( 1 + \frac{1}{\deltamin} \right) \approx \frac{1}{|\setA_i^{\delta}|}.$}

Combining the two inequalities \eqref{eqn:tilde_to_hat} and \eqref{eqn:tilde_to_true} using the triangle inequality, and observing that $|\setB_i^{\delta}| \leq \ktrue - |\setA_i^{\delta}|$, we complete the proof of Proposition \ref{prop:small_bdr2}.
